# Supplementary material for: Neuro-Symbolic World Models for Adapting to Open World Novelty
Source: arXiv:2301.06294 source file (2023-01-16)
Supplement: Supplementary file 1 [file 9_appendix.tex]

%Optionally include extra information (complete proofs, additional experiments and plots) in the appendix.
%This section will often be part of the supplemental material.

\section*{Appendix A: Societal Impacts}

Reinforcement learning is a general purpose and capable class of algorithms that can be applied to sequential decision-making problems, from computer games to logistics to robotics. 
While our current experiments are limited to feasibility studies in gridworld environments, our technique may eventually scale to richer, more complex environments. 
These include agents that can play online games that are periodically patched or use ``house rules''~\cite{peng2021detecting}, or household robotics where everyday life presents numerous novelties.
Our proposed technique is most appropriately geared toward situations where novelties occur and there is no option to re-train the agent from scratch. 
This includes dynamic command and control operations against an adversary with potentially unknowable capabilities, which can include military operations and also cybersecurity protection.
Novelty-handling could also be useful in domains such as healthcare and financial trading, where responsiveness is important.
These potential benefits make this line of research---of which this paper is just an early step---important.

One purpose of ``societal impacts'' statements such as this is to put in writing our express desire that technologies that derive directly or indirectly from this work not be used for offensive military purposes or other uses that are detrimental to human well-being or degrade civil rights.  
This statement is provided so that future application developers cannot claim lack of awareness of societal implications and our intentions.

\section*{Appendix B: Training Details}

\mark{Did you specify all the training details (e.g., data splits, hyperparameters, how they
were chosen)? Did you include the total amount of compute and the type of resources used (e.g., type
of GPUs, internal cluster, or cloud provider)?}

\section*{Appendix B: Experimental Details}

There exist several environments that require deployment-time novelty detection, characterization, and adaptation for games such as Monopoly~\cite{kejriwal2021multi}, Angry Birds~\cite{gamagenovelty}, and grid worlds~\cite{goel2021novelgridworlds, balloch2022novgrid}.

\Mark{Show images of the grid worlds we used}

\begin{figure*}[ttt!]
%\begin{minipage}[t]{0.39\textwidth}
\begin{algorithm}[H] 
% \scriptsize
\SetAlgoLined
\KwIn{$D(), \epsilon>0, R, G, s, a, s' $}
\KwOut{$R^{*}$}
$C \leftarrow []$\;

$P \leftarrow P \cup [R,\infty]$\; 

$d* = \infty$\;

\While{$P \ne \emptyset$}{
    $\hat{R} \sim P$\;
    
    $d = D(\hat{R}, s, a, s')$\;
    
    \eIf{$d < \epsilon$ }{
        return $R^{*}$\;}{
        $N = C \cap \mathbf{PotentialRule}(\hat{R}, G)$\;
        
        $P \leftarrow P \cup (N \oplus [\cdot,d])$\;
        
        \eIf{$d* > d$}{
            $C \leftarrow C \cup R$\;
            
            $R \leftarrow \hat{R}$\;
            
            $d* \leftarrow d$\;
            }{
            $C \leftarrow C \cup \hat{R}$\;}
        }
    }
$R^{*} = \hat{R}$\;
\caption{Rule Model Update}
\label{alg:rule-learning}
\end{algorithm}
%\end{minipage}
%\hfill
\caption{\Mark{algo 1 is impossible to follow without more descriptive variable names. Also we may want to move both algos to the appendix, in which case add comments.}}
\label{fig:rule-learner}
\end{figure*}
\begin{figure*}
%\begin{minipage}[t]{0.60\textwidth}
\begin{algorithm}[H] 
% \scriptsize
\SetAlgoLined
\KwIn{Pre-Novelty Policy $\pi_{0}$, Rule Model $M$, Env $E$, Convergence Criteria $c$, State $s_{t}$}
\KwOut{Post-Novelty Policy $\pi_{\rm post}$}
Select action $a_{t}=\pi_{0}(s_{t})$ \;

Predict next state $\hat{s}_{t+1} = M(s_{t}, a_{t})$ \;

Execute $a_{t}$ and observe 
%next state and reward 
$s_{t+1}, r_{t}=Env(a_{t})$ \;

\If{$DetectNovelty(\hat{s}_{t+1}, s_{t+1})=True$}
    {
    $\pi_{\rm post} \leftarrow \pi_0$\;
    
    \While{Prediction error $\lVert \hat{s}_{t+1} - s_{t+1} \rVert^{2}_{2} > c$}{
        $RolloutBuffer \leftarrow MixRatio \times CollectRollouts(\pi_{\rm post})$\;
        
        $UpdateGameCloning$ \;
        
        $RolloutBuffer \leftarrow (1 - MixRatio) \times ImagineRollouts(M)$\; %RuleModel.ImagineRollouts()$ \;

        $\pi_{\rm post} \leftarrow$ update $\pi_{\rm post}$ with $RolloutBuffer$ \;
    }
    }
\caption{Imagination-Based Adaptation}
\label{alg:imagination-based adaptation}
\end{algorithm}
%\end{minipage}
% \hfill
 \caption{\Mark{Question about alg 2 while-statement. Does this still allow realtime execution? Wonder if we should make alg 2 the whole execution loop with pre-novelty and post-novelty mixing?} \jb{Good point. My thinking was that the "while" loop was the "real time", so we would be always operating in real time, but while it was unconverged we were learning}}
\end{figure*}
